# Supplementary material for: On the Uncertainty Estimates of Equivariant-Neural-Network-Ensembles Interatomic Potentials
Source: arXiv:2309.00195 ancillary file (2023-09-01)
Supplement: Supplementary file 1 [file EquivariantEnsemble_silicon-SI.pdf]

# Critical assessment on the robustness of uncertainty estimates in ensembles of deep-learning potentials

## Electronic Supplementary Information

Shuaihua Lu<sup>1,2</sup>, Luca Ghiringhelli<sup>3,1</sup>, Christian Carbogno<sup>1</sup>, Jinlan Wang<sup>2</sup>, and Matthias Scheffler<sup>1</sup>

<sup>1</sup> *The NOMAD Laboratory at the Fritz Haber Institute of the Max-Planck-Gesellschaft and IRIS Adlershof of the Humboldt-Universität zu Berlin, Germany;*

<sup>2</sup> *School of Physics, Southeast University, Nanjing, China;*

<sup>3</sup> *Physics Department and IRIS Adlershof of the Humboldt-Universität zu Berlin, Germany*

*\*email:*

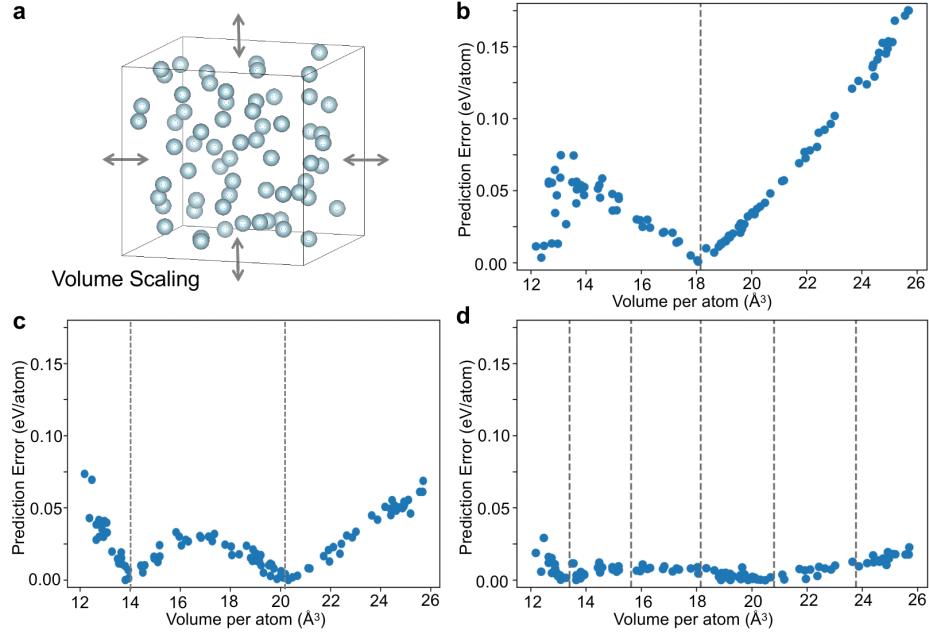

FIG. 1. The results of density testing for liquid silicon. (a) Schematic diagrams of silicon configurations at different densities, obtained by proportionally increasing/decreasing the volume. The actual error of NNP when the training set contains (a) one density, (b) two densities, and (c) five densities of silicon configurations. The dashed line represents the density of the silicon configurations in the training set.

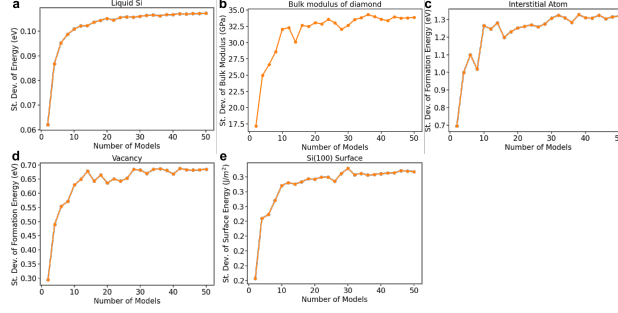

FIG. 2. The relationship between the size of the neural network potential (NNP) ensemble model and its uncertainty. (a) Liquid silicon, (b) bulk modulus of the diamond phase of silicon, (c) silicon interstitial, (d) silicon vacancy, and (e) Si (100) surface.

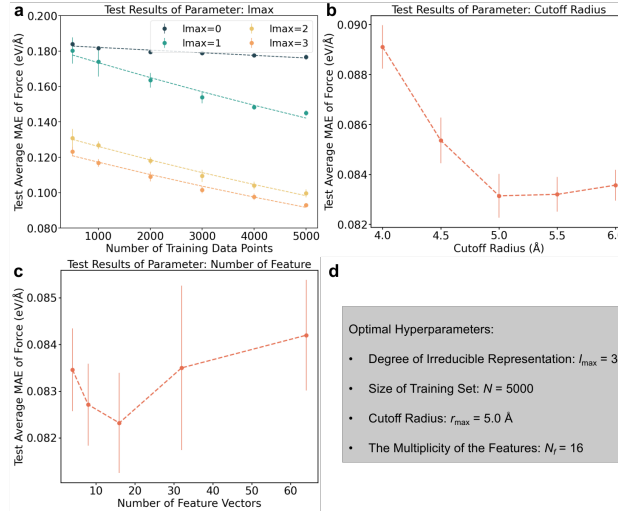

FIG. 3. The results of NequIP hyperparameter optimization and training set size optimization. (a) Log-log plot of the predictive error on the test set of liquid silicon from using NequIP with  $l_{max} \in \{0, 1, 2, 3\}$  as a function of training set size, measured via the force MAE. (b) The cutoff radius and (c) the multiplicity of the features, are optimized. The results show that the optimal feature dimension is 16 and the optimal cutoff radius distance is 5.0 Å for liquid silicon. (d) The optimal values of hyperparameters for NequIP

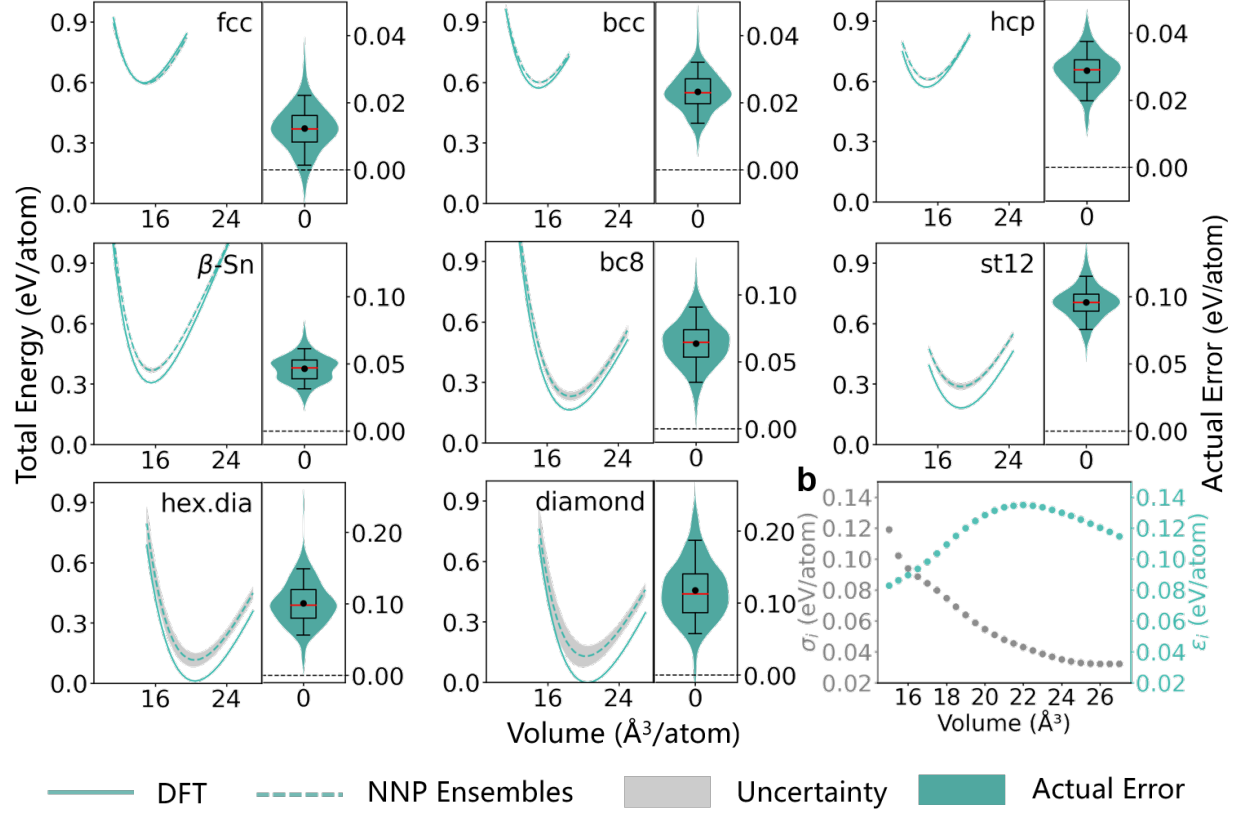

FIG. 4. Energy per atom vs volume per atom for various bulk crystal structures computed using the DFT (solid lines) and the NNP ensemble model (dashed lines), and the gray area depicts one standard deviation from the mean. Distribution of test-set actual errors for 8 sets of bulk crystal structures. The black dot represents the mean actual error, the orange lines are the median actual error, the boxes are the quartiles, and the whiskers are the 5% and 95% actual error.

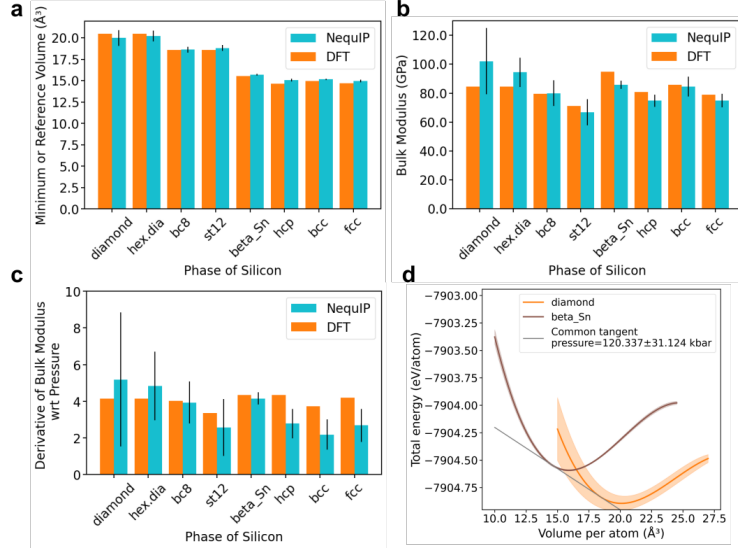

FIG. 5. The prediction results of NNP ensembles for structures of 8 solid phases, including (a) minima positions (equilibrium volume), (b) curvatures (bulk modulus), (c) derivative of bulk modulus with respect to pressure and (d) transition pressure between diamond silicon and  $\beta$ -Sn silicon. The error bar is the standard deviation.

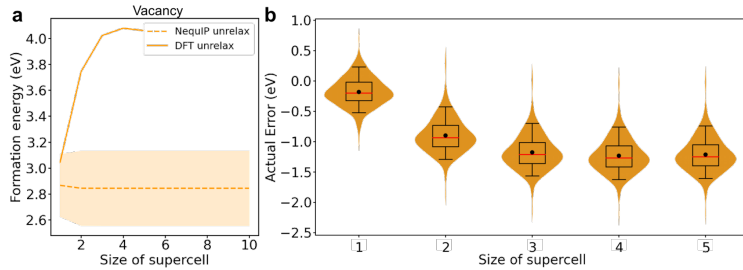

FIG. 6. (a) Analysis of the actual errors for the vacancy with various supercell sizes. The solid line is the formation energy computed using the DFT (solid lines) from the unrelaxed crystal structure. The dashed line is the formation energy computed using the NNP ensemble model. The colour area depicts the uncertainty. (b) The distribution of actual errors for the vacancy with various supercell sizes. The black dot represents the mean actual error, the red lines are the median actual error, the boxes are the quartiles, and the whiskers are the 5% and 95% actual error.

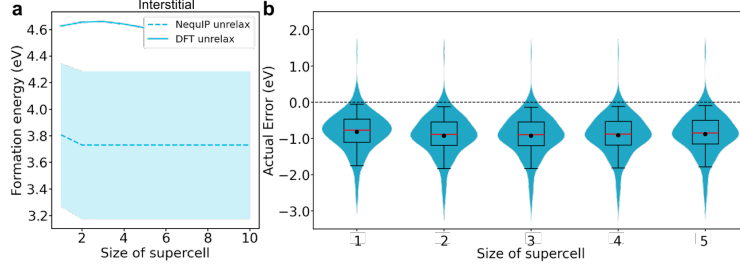

FIG. 7. (a) Analysis of the actual errors for the interstitial with various supercell sizes. The solid line is the formation energy computed using the DFT (solid lines) from the unrelaxed crystal structure. The dashed line is the formation energy computed using the NNP ensemble model. The colour area depicts the uncertainty. (b) The distribution of actual errors for the interstitial with various supercell sizes. The black dot represents the mean actual error, the red lines are the median actual error, the boxes are the quartiles, and the whiskers are the 5% and 95% actual error.

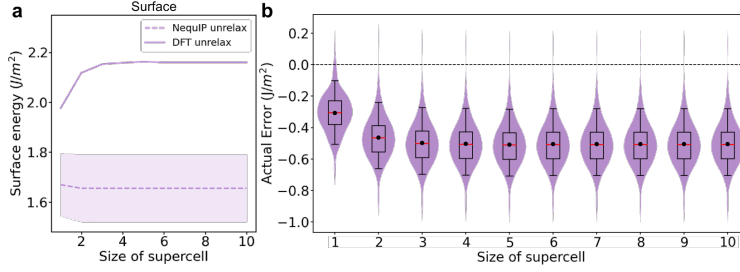

FIG. 8. (a) Analysis of the actual errors for the Si (100) surface with various supercell sizes. The solid line is the surface energy computed using the DFT (solid lines) from the unrelaxed crystal structure. The dashed line is the surface energy computed using the NNP ensemble model. The colour area depicts the uncertainty. (b) The distribution of actual errors for the Si (100) surface with various supercell sizes. The black dot represents the mean actual error, the red lines are the median actual error, the boxes are the quartiles, and the whiskers are the 5% and 95% actual error.

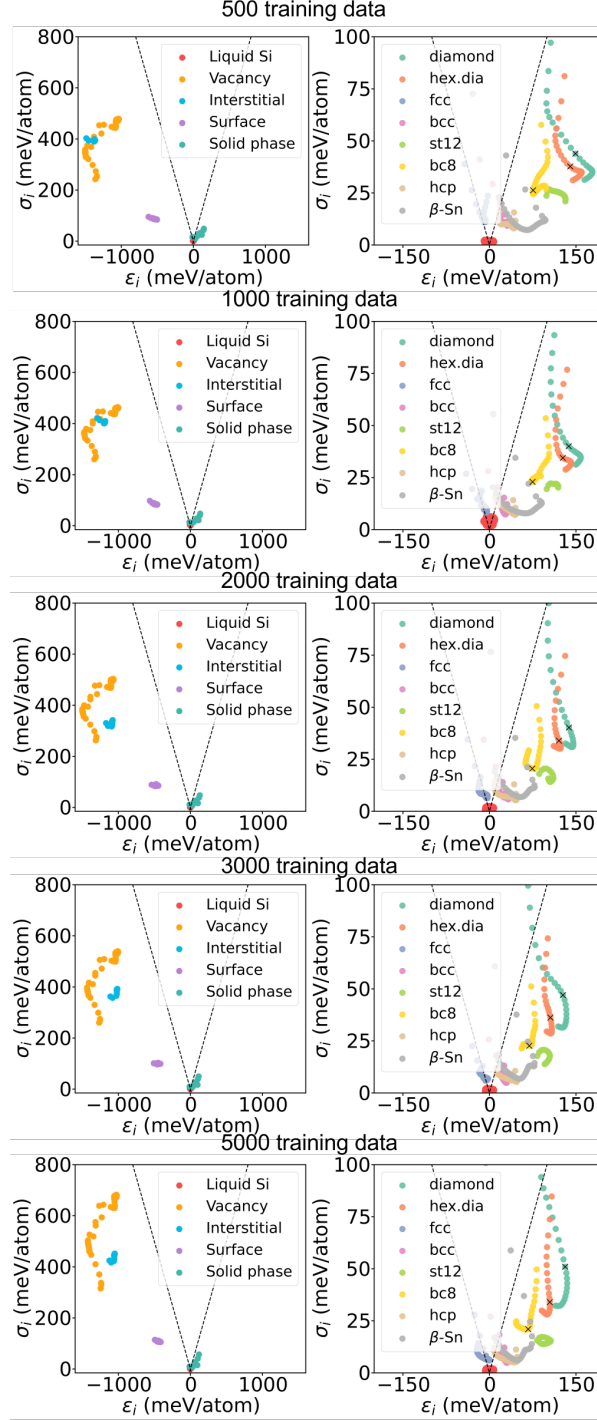

FIG. 9. The ensemble uncertainty  $\sigma$  is plotted against the actual error  $\epsilon$ , calculated as the difference between the predicted value from NNP ensembles trained on various sizes of the training data set and the DFT calculated value for five test sets, including liquid silicon, bulk crystal structures, Si vacancy, Si interstitial atom and Si(100) surface. The dashed line represents the ideal relationship between the actual error and uncertainty,  $\sigma = \pm \epsilon$ . The crosses mark the minimum energy structure (according to the NNP ensembles) in the equations of state or geometry optimization

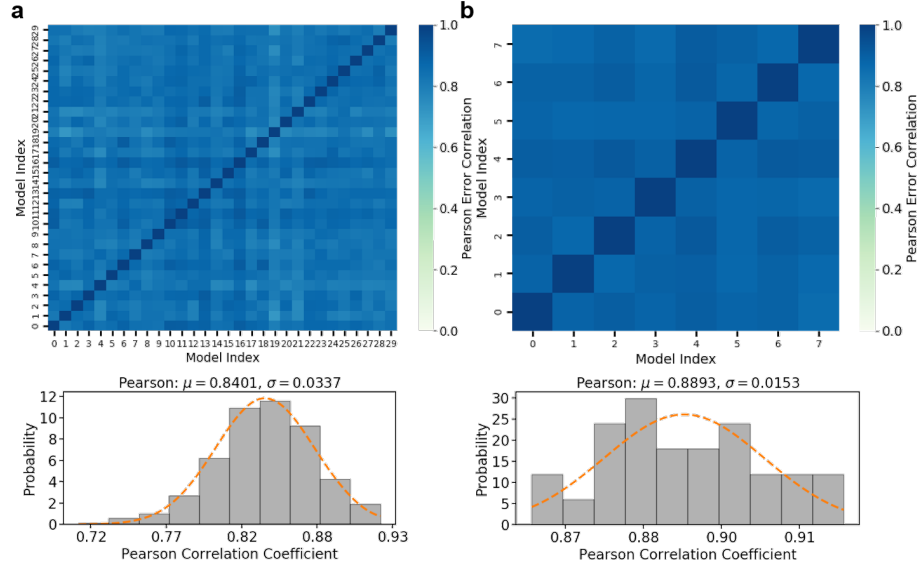

FIG. 10. Pearson pair correlation of the error vectors for the liquid test set (1 000 configurations) for (left) models with the same training set and different initial guess of the NN parameters and (right) different training set, where each model is an ensemble over the different initial guesses.
